# Supplementary material for: Long-Term Dynamic Window Approach for Kinodynamic Local Planning in Static and Crowd Environments
Source: arXiv:2310.02648 source file (2023-10-04)
Supplement: Supplementary file 1 [file appendix.tex]

\section{APPENDIX}

This appendix gives the values of all parameters in the proposed method for the experiments, which are shown in Tab.~\ref{tab:value}.

\begin{table}[htbp]
    \centering
    
    \fontsize{8}{8}\selectfont
    \begin{threeparttable}
        \caption{values of all parameters in the proposed method for the experiments.} 
        \label{tab:value}
        \setlength{\tabcolsep}{4pt}
        \begin{tabular}{>{\centering\arraybackslash}p{0.5\linewidth}>{\centering\arraybackslash}p{0.2\linewidth}>{\centering\arraybackslash}p{0.2\linewidth}}
        \toprule
        Parameter Meaning & Symbol & Value \cr
        \midrule
        \midrule
        \addstackgap[4pt] Number of frames & $N$ & 15 \cr
        \addstackgap[4pt] Time segment & $\Delta T$ & 0.2 \cr
        \addstackgap[4pt] Distance field weight & $w_\mathrm{do}$ & 600.0 \cr
        \addstackgap[4pt] Distance field weight & $w_\mathrm{db}$ & 200.0 \cr
        \addstackgap[4pt] Distance field parameter & $\eta$ & 0.3 \cr
        \addstackgap[4pt] Distance field parameter & $\beta$ & 1.0 \cr
        \addstackgap[4pt] Velocity space sampling parameter & $V$ & 8 \cr
        \addstackgap[4pt] LT-DWA parameter & $K^{'}$ & 400 \cr
        \addstackgap[4pt] Voxel sampling parameter & $W$ & 12 \cr
        \addstackgap[4pt] Decline rate & $\gamma$ & 0.9 \cr
        \addstackgap[4pt] Safety cost weight & $w_\mathrm{c}$ & 1.0 \cr
        \addstackgap[4pt] Navigation cost weight & $w_\mathrm{no}$ & 5.0 \cr
        \addstackgap[4pt] Navigation cost weight & $w_\mathrm{na}$ & 1.0 \cr
        \addstackgap[4pt] Navigation cost weight & $w_\mathrm{nt}$ & 0.5 \cr
        \addstackgap[4pt] Navigation cost weight & $w_\mathrm{nv}$ & 0.1 \cr
        \addstackgap[4pt] Stability cost weight & $w_{\omega}$ & 0.1 \cr
        \addstackgap[4pt] Stability cost weight & $w_{a_v}$ & 0.1 \cr
        \addstackgap[4pt] Stability cost weight & $w_{a_{\omega}}$ & 0.1 \cr
        \bottomrule
        \end{tabular}
    \end{threeparttable}
\end{table}
